# Supplementary material for: Spacerini: Plug-and-play Search Engines with Pyserini and Hugging Face
Source: arXiv:2302.14534 source file (2024-03-24)
Supplement: Supplementary file 1 [file emnlp23-demo-hf-spacerini-appendix.tex]

\section{Requesting additional disk space}\label{sec:disk_flow}

Hugging Face Spaces allow users to choose from a variety of backend options,\footnote{\url{https://hf.co/docs/hub/spaces-overview\#hardware-resources}} with basic, free variants and more powerful paid alternatives. Academic users are encouraged to apply for community grants which can result in granting access to free, upgraded backend machines.\footnote{\url{https://hf.co/docs/hub/spaces-gpus}} In order to apply, one can navigate to the \texttt{Settings} tab in their Space and click on the \texttt{Apply for a community GPU grant} highlighted text. As demonstrated in Figure~\ref{fig:disk_request}, this will open a pop-up window where users can describe their use cases and backend demands. The applications are evaluated on a case-by-case basis. Given that Spaces are primarily intended for hosting Machine Learning demos, GPU provisioning takes the front seat; however, readers are welcome to submit their disk space requests via the same flow.

\begin{figure}
\centering
\includegraphics[width=\columnwidth]{figures/disk_request_flow.pdf}
\caption{Additional disk space request flow.}
\label{fig:disk_request}
\end{figure}
